# Supplementary material for: Towards Vision Mixture of Experts for Wildlife Monitoring on the Edge
Source: arXiv:2411.07834 source file (2024-11-12)
Supplement: Supplementary file 1 [file appendix_a.tex]

\section*{Appendix}
\label{sec:appendix_a}

% \section{Sample expert groupings of inaturalist birds species}

\section{Sample expert groupings of imagenet image patches}

\begin{figure*}[ht!]
    \begin{center}
        \begin{tabular}{llll}
            \includegraphics[width=.28\linewidth]{Styles/figures/placeholder_imagenet/birds_cluster.PNG} & \includegraphics[width=.28\linewidth]{Styles/figures/placeholder_imagenet/cat_cluster.PNG} & \includegraphics[width=.28\linewidth]{Styles/figures/placeholder_imagenet/dog_cluster.PNG}\\
            \includegraphics[width=.28\linewidth]{Styles/figures/placeholder_imagenet/reptile_cluster.PNG} & \includegraphics[width=.28\linewidth]{Styles/figures/placeholder_imagenet/human_cluster.PNG} & \includegraphics[width=.28\linewidth]{Styles/figures/placeholder_imagenet/fruits_cluster.PNG}\\
            \includegraphics[width=.28\linewidth]{Styles/figures/placeholder_imagenet/text_cluster.PNG} & \includegraphics[width=.28\linewidth]{Styles/figures/placeholder_imagenet/building_cluster.PNG} & \includegraphics[width=.28\linewidth]{Styles/figures/placeholder_imagenet/vehicle_cluster.PNG}\\
            \end{tabular}
    \caption{ Sample patches assigned to different MoE-16 experts in the last MoE layer after finetuning the model on imagenet. The presented patches that are routed to different expert generally include species, text and structures that are either semantically similar or have similar visual features.}
    \label{fig:imagenet_semantic_splits}
    \end{center}
\end{figure*}

\section{Routing affinity for the every other layer Mixture of Experts model.}

\begin{figure*}[ht!]
\begin{center}
    \begin{tabular}{cccc}
        \includegraphics[width=.22\linewidth]{Styles/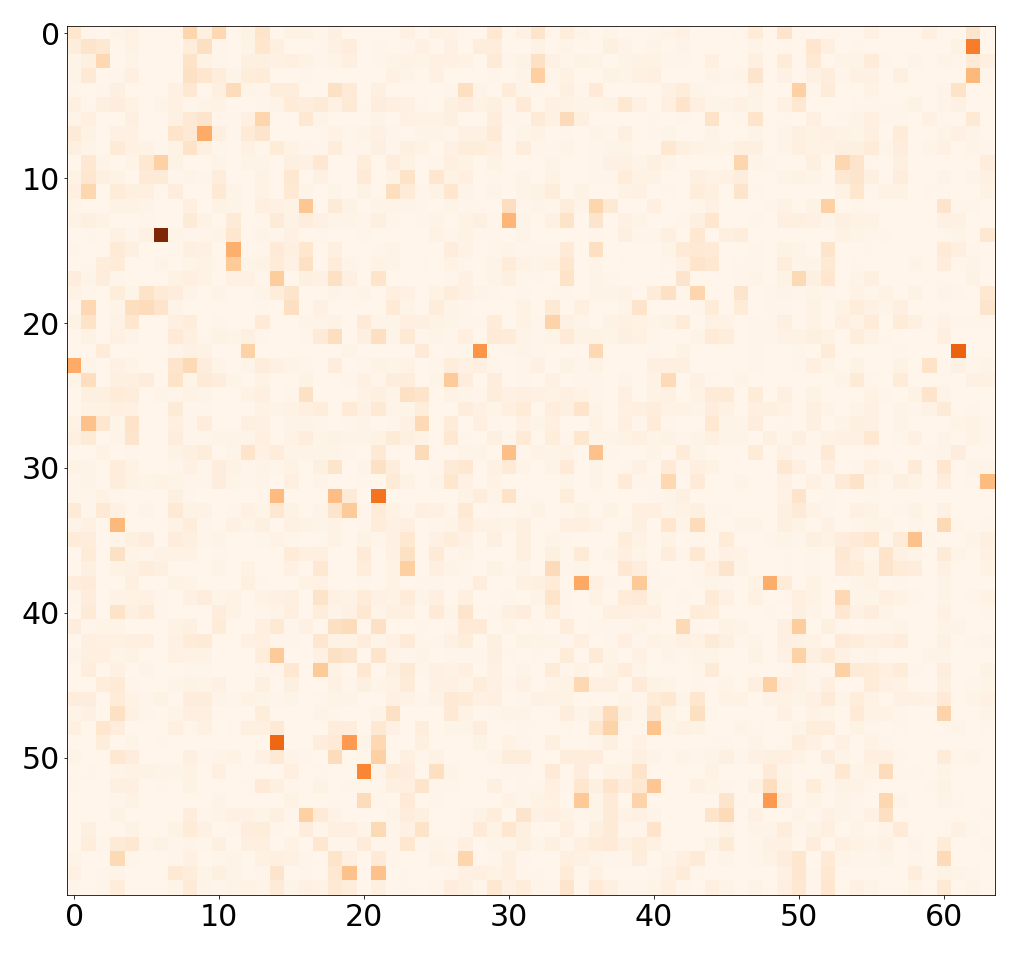} &

        \includegraphics[width=.22\linewidth]{Styles/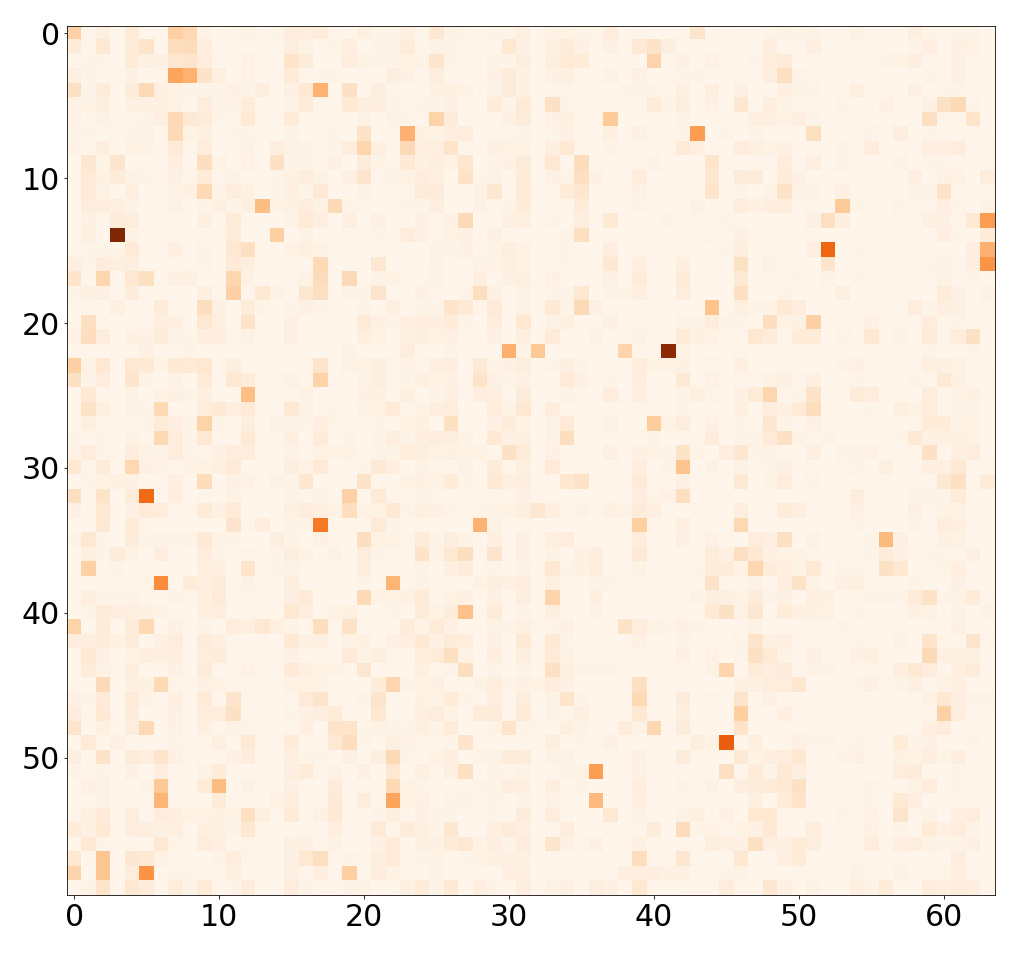} &
        
        \includegraphics[width=.22\linewidth]{Styles/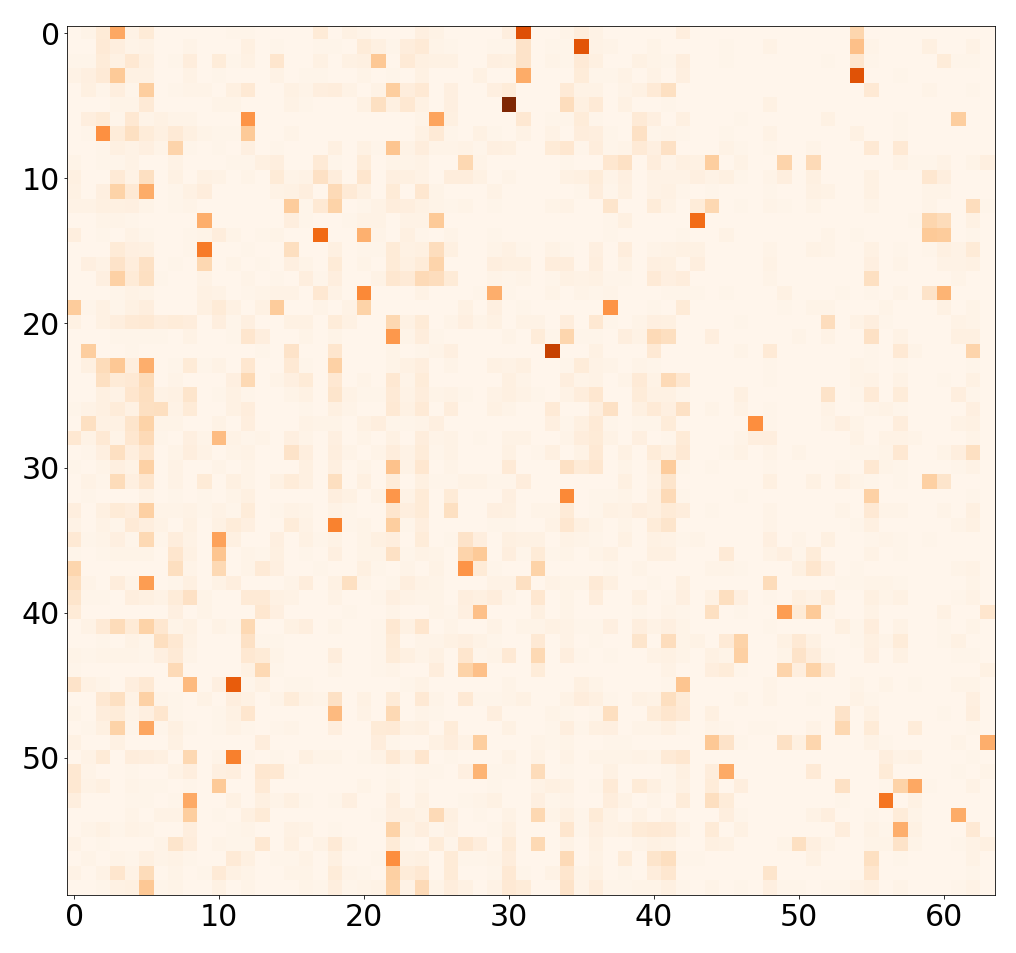} & 
        
        \includegraphics[width=.22\linewidth]{Styles/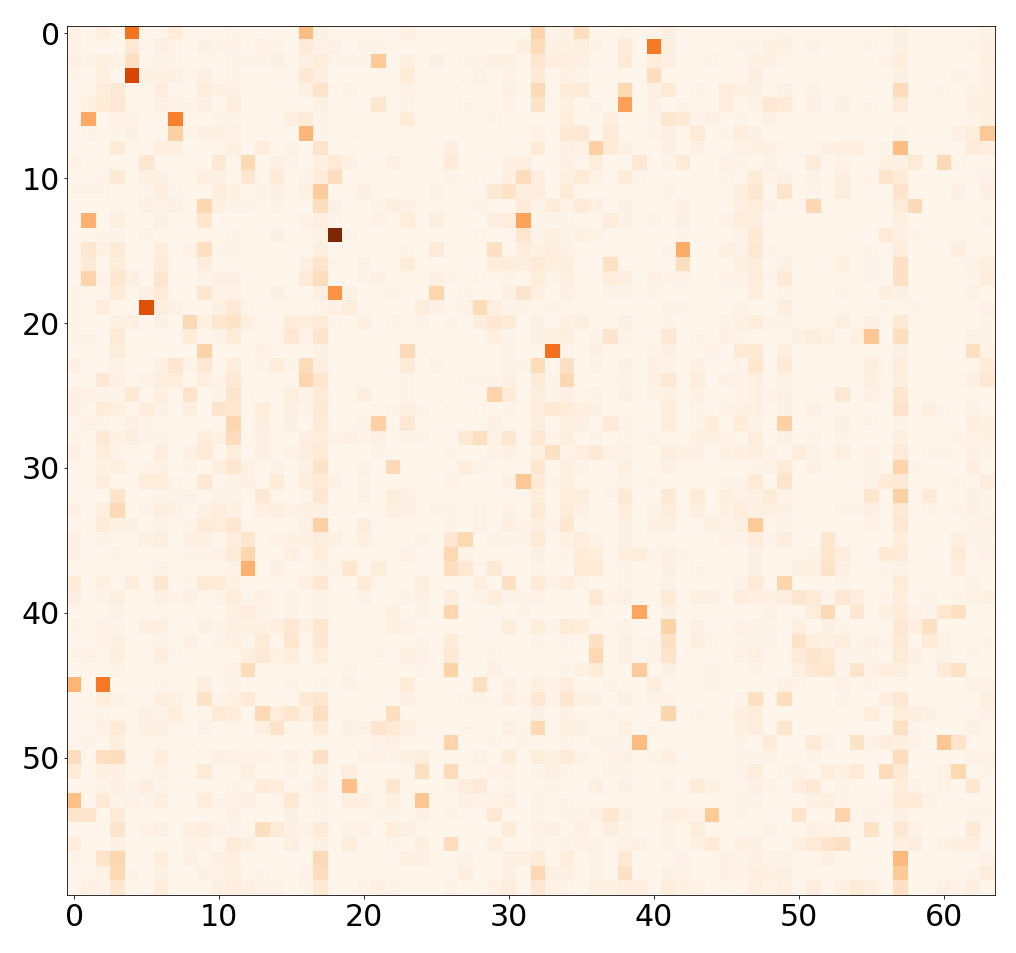}  \\
        
        % $(a)$ & $(b)$ & $(c)$ & $(d)$ \\
    \end{tabular}
    \caption{Cluster-class affinity using softmax temperature of $0.001$ and cut-off threshold of $0.05$ for layers $2,4,6,8$ in order for mobilevit-0.5 with 64 experts for each reported layer.}
    \label{fig:affinity_2468}
\end{center}
\end{figure*}

% \section{Routing success of image vs audio tokens}
% We might have to include this in the supplemental material submission

% \section{Sample attention context in MobileViTMoE layer 8}
% \begin{center}
% \begin{tabular}{llll}
% Label 1 & \includegraphics[width=.2\linewidth,valign=m]{images/context_1.png} & \includegraphics[width=.2\linewidth,valign=m]{images/context_2.png} & \includegraphics[width=.2\linewidth,valign=m]{images/context_3.png}\\
% Label 2 & \includegraphics[width=.2\linewidth,valign=m]{images/context_4.png} & \includegraphics[width=.2\linewidth,valign=m]{images/context_1.png} & \includegraphics[width=.2\linewidth,valign=m]{images/context_2.png}\\

% \end{tabular}
% \captionof{figure}{ Placeholder for sample context vectors after pretraining with audioset. Pick some of the more challenging ones to compare across algorithms}
% \end{center}

% \begin{center}
% \begin{tabular}{llll}
% Label 1 & \includegraphics[width=.85\linewidth,valign=m]{images/sample_aud.png}
% \end{tabular}
% \captionof{figure}{ Placeholder for audio attention context map.}
% \end{center}
%%%%%%%%%%%%%%%%%%%%%%%%%%%%%%%%%%%%%%%%%%%%%%%%%%%%%%%%%%%%
